# Supplementary material for: Hyperfine Structure of Transition Metal Defects in SiC
Source: arXiv:2104.12351 ancillary file (2021-04-26)
Supplement: Supplementary file 1 [file supplemental_material.pdf]

# Supplemental Material: Hyperfine Structure of Transition Metal Defects in SiC

Benedikt Tissot* and Guido Burkard†
*Department of Physics, University of Konstanz, D-78457 Konstanz, Germany*

## DERIVATION OF $H_{\mathrm{hf}}$

In this section of the supplemental material we show a more indepth derivation of the general form of the hyperfine Hamiltonian of a spin-orbit coupled electron state in a $D$-shell of a transition metal (TM) defect in a crystal environment with $C_{3v}$ symmetry with the TM nuclear spin. We start by writing the hyperfine Hamiltonian with the non-trivial scalar products expanded

$$\begin{aligned} H_{\mathrm{hf}} = a_{\mathrm{FC}}\vec{S}\cdot\vec{I} - 3a\Bigg\{ &\left[\left(-\frac{y^2-x^2}{2}S_x + xyS_y\right) + xzS_z + \frac{y^2+x^2}{2}S_x - S_x/3 + L_x/3\right] I_x \\ &+ \left[\left(\frac{y^2-x^2}{2}S_y + xyS_x\right) + yzS_z + \frac{y^2+x^2}{2}S_y - S_y/3 + L_y/3\right] I_y \\ &+ \left[(xzS_x + yzS_y) + z^2S_z - S_z/3 + L_z/3\right] I_z \Bigg\}, \end{aligned} \tag{S1}$$

where $(x,y,z)^T = \vec{r}/r$ are the direction vector components of the position $\vec{r}$ of the electron relative to the TM nucleus in the origin. In the Appendices of [S1] we discussed the application of the Wigner-Eckart theorem for the given symmetry in detail; Analogously we use the eigenbasis of the crystal potential inside the $d$-orbital made up of two doublets $|\pm\rangle_i$ given by admixtures of the states $|l=2, m\neq 0\rangle$ and a singlet $|0\rangle = |l=2, m=0\rangle$. For the hyperfine Hamiltonian (S1) the relevant operators are the square components $kl$ with $k,l = x,y,z$ acting on the orbital states. These components can be mapped to operators that transform the same as $x,y,z$, implying a one-to-one correspondence of the application of the Wigner-Eckart theorem to the orbital terms of $V_{\mathrm{el}}$. In particular, $z^2$ and $(x^2+y^2)/2$ transform like $z$ according to the irrep $A_1$, while $\{zx, zy\}$ and $\{(y^2-x^2)/2, xy\}$ transform like $\{x,y\}$ according to the irrep $E$. The orbital operators transforming like $z$ have the form

$$\mathcal{Z}_{12}\Big(\sum_{\sigma=\pm} |\sigma_1\rangle\langle\sigma_2| + \mathrm{h.c.}\Big) + \sum_{i=1,2,3} \mathcal{Z}_{ii}P_i \tag{S2}$$

where $P_j = |+_j\rangle\langle +_j| + |-_j\rangle\langle -_j|(\ j=1,2\ )$ and $P_3 = |0\rangle\langle 0|$. The operators transforming like $x$ have the form

$$\sum_{i,j=1,2} \mathcal{X}_{ij}(|+_i\rangle\langle -_j| + \mathrm{h.c.}) + \sum_{i=1,2} \mathcal{X}_{i3}(|+_i\rangle\langle 0| - |-_i\rangle\langle 0| + \mathrm{h.c.}) \tag{S3}$$

and the corresponding operator transforming like $y$

$$\sum_{i,j=1,2} \mathcal{X}_{ij}(\mathrm{i}\,|+_i\rangle\langle -_j| + \mathrm{h.c.}) + \sum_{i=1,2} \mathcal{X}_{i3}(\mathrm{i}\,|+_i\rangle\langle 0| + \mathrm{i}\,|-_i\rangle\langle 0| + \mathrm{h.c.}). \tag{S4}$$

While all operators transforming like $y$ have this form, the parameters $\mathcal{X}_{ij}$ and $\mathcal{Z}_{ij}$ vary. The $\vec{L}$ operators take the form discussed in [S1].

Because the spin-orbit interaction is much larger than the hyperfine interaction, we first approximately diagonalize the spin-orbit Hamiltonian, using the first-order Schrieffer-Wolff transformation we derived in [S1], given in terms of approximate eigenstates (rows of $1 - S_{so,1}$)

$$|i,\Gamma_{5/6},\sigma\rangle^{(1)} = |\sigma_i\rangle|\sigma\rangle + \sigma\frac{2\lambda_{\perp,12}r_{\parallel,12}}{(\epsilon_2-\epsilon_1)(g_s+2r_{\parallel,ii})}|-\sigma_i\rangle|-\sigma\rangle - \frac{(-1)^i\lambda_{\parallel,12}}{2\,(\epsilon_2-\epsilon_1)}|\sigma_{3-i}\rangle|\sigma\rangle - \frac{\sigma\lambda_{\perp,12}}{\epsilon_2-\epsilon_1}|-\sigma_{3-i}\rangle|-\sigma\rangle\,, \tag{S5}$$

$$|i,\Gamma_4,\sigma\rangle^{(1)} = |-\sigma_i\rangle|\sigma\rangle - \frac{(-1)^i\lambda_{\parallel,12}}{2\,(\epsilon_2-\epsilon_1)}|-\sigma_{3-i}\rangle|\sigma\rangle - \frac{\sigma\lambda_{\perp,i3}}{\epsilon_3-\epsilon_i}|0\rangle|-\sigma\rangle \ \text{ for } i<3 \text{ and} \tag{S6}$$

$$|3,\Gamma_4,\sigma\rangle^{(1)} = |0\rangle|\sigma\rangle + \frac{\sigma\lambda_{\perp,13}}{\epsilon_3-\epsilon_1}|\sigma_1\rangle|-\sigma\rangle + \frac{\sigma\lambda_{\perp,23}}{\epsilon_3-\epsilon_2}|\sigma_2\rangle|-\sigma\rangle\,, \tag{S7}$$

with $\epsilon_j, \epsilon_3$ ($j = 1, 2$) the eigenvalues with the eigenvectors $|\pm_j\rangle, |0\rangle$ of the crystal potential and $\lambda_{k,ij}$ the spin-orbit parameters.

With the Schrieffer-Wolff transformation we can approximate the Hamiltonian $H$ [Eq. (1) of the main text] with an effective Hamiltonian $H_{\rm eff} = \sum_{i=1,2,3} P_i(H + [S_{\rm so,1}, H])P_i = H_{\rm so}^{\rm eff} + H_{\rm hf}^{\rm eff} + H_{z,\rm nuc}$. Renaming the independent (combinations of) parameters we find

$$\begin{aligned} H_{\rm so}^{\rm eff} = &\sum_{i,\Gamma_\gamma} H_{i,\Gamma_\gamma}^{\rm KD} \\ &+ \sum_{j,\sigma} \frac{\mu_B}{2} \Big[ g_{j,c}(\sigma B_x + iB_y) |j, \Gamma_{5/6}, \sigma\rangle \langle j, \Gamma_4, \sigma| \\ &+ g_{f,c}(B_x - \sigma i B_y) |j, \Gamma_{5/6}, \sigma\rangle \langle j, \Gamma_4, -\sigma| + \text{h.c.}\Big]. \end{aligned} \tag{S8}$$

with the KD Hamiltonians $H_{i,\Gamma_\gamma}^{\rm KD}$ from Eq. (3) of the main text and

$$\begin{aligned} H_{\rm hf}^{\rm eff} = &\sum_{i,\Gamma_\gamma} H_{{\rm hf,KD},i,\Gamma_\gamma} \\ &+ \sum_{j,\sigma} a_{j,c}[(\sigma I_x + {\rm i} I_y) |j, \Gamma_{5/6}, \sigma\rangle \langle j, \Gamma_4, \sigma| + \text{h.c.}] \\ &+ \sum_{j,\sigma} a_{j,f}[(I_x - \sigma {\rm i} I_y) |j, \Gamma_{5/6}, \sigma\rangle \langle j, \Gamma_4, -\sigma| + \text{h.c.}]. \end{aligned} \tag{S9}$$

with the diagonal blocks

$$H_{{\rm hf,KD},j,\Gamma_{5/6}} = \frac{1}{2}\left( a^{\parallel}_{j,\Gamma_{5/6}} \sigma^z_{j,\Gamma_{5/6}} + a^{\perp}_{j,\Gamma_{5/6}} \sigma^x_{j,\Gamma_{5/6}} \right) I_z, \tag{S10}$$

$$H_{{\rm hf,KD},j,\Gamma_4} = \frac{a^{\parallel}_{j,\Gamma_4}}{2} \sigma^z_{j,\Gamma_4} I_z + \frac{a^{\perp}_{j,\Gamma_4}}{2} (\sigma^x_{j,\Gamma_4} I_x - \sigma^y_{j,\Gamma_4} I_y), \tag{S11}$$

$$H_{{\rm hf,KD},3,\Gamma_4} = \frac{a^{\parallel}_{3,\Gamma_4}}{2} \sigma^z_{3,\Gamma_4} I_z + \frac{a^{\perp}_{3,\Gamma_4}}{2} (\sigma^x_{3,\Gamma_4} I_x + \sigma^y_{3,\Gamma_4} I_y), \tag{S12}$$

for $j = 1, 2$, and $\sigma^k_{i,\Gamma_\gamma}$ is the $k$ Pauli matrix acting between the pseudo-spin states of the $i, \Gamma_\gamma$ KD. Analogously we can write the above equations using coupling tensors $H_{{\rm hf,KD},i,\Gamma_\gamma} = \frac{1}{2} \vec{\sigma}_{i,\Gamma_\gamma} \cdot A_{i,\Gamma_\gamma} \cdot \vec{I}$, with

$$A_{j,\Gamma_{5/6}} = \begin{pmatrix} 0 & 0 & a^{\perp}_{j,\Gamma_{5/6}} \\ 0 & 0 & 0 \\ 0 & 0 & a^{\parallel}_{j,\Gamma_{5/6}} \end{pmatrix}, A_{j,\Gamma_4} = \begin{pmatrix} a^{\perp}_{j,\Gamma_4} & 0 & 0 \\ 0 & -a^{\perp}_{j,\Gamma_4} & 0 \\ 0 & 0 & a^{\parallel}_{j,\Gamma_4} \end{pmatrix}, A_{3,\Gamma_4} = \begin{pmatrix} a^{\perp}_{3,\Gamma_4} & 0 & 0 \\ 0 & a^{\perp}_{3,\Gamma_4} & 0 \\ 0 & 0 & a^{\parallel}_{3,\Gamma_4} \end{pmatrix}. \tag{S13}$$

## DIAGONALIZATION FOR A MAGNETIC FIELD ALONG THE CRYSTAL AXIS

In the main text we showed how to approximate the effective Hamiltonian derived in the previous section with a block diagonal one [see Eq. (13) in the main text]. Inside the blocks corresponding to the different KDs we find that, even including the hyperfine interaction up to second order, the nuclear KD Hamiltonians can be decomposed into $2 \times 2$ blocks for a magnetic field $\vec{B}$ along the crystal axis. For the $j, \Gamma_{5/6}$ states the blocks are spanned by $|j, \Gamma_{5/6}, \uparrow\rangle |m_I\rangle, |j, \Gamma_{5/6}, \downarrow\rangle |m_I\rangle$, for the $j = 1, 2, \Gamma_4$ states by $|j, \Gamma_4, \uparrow\rangle |m_I\rangle, |j, \Gamma_4, \downarrow\rangle |m_I - 1\rangle$(the states $|j, \Gamma_4, \uparrow\rangle |-I\rangle, |j, \Gamma_4, \downarrow\rangle |I\rangle$ are already diagonal), and for $3, \Gamma_4$ states by $|3, \Gamma_4, \uparrow\rangle |m_I\rangle, |3, \Gamma_4, \downarrow\rangle |m_I + 1\rangle$ (the states $|3, \Gamma_4, \uparrow\rangle |I\rangle, |3, \Gamma_4, \downarrow\rangle |-I\rangle$ are already diagonal). We can diagonalize the non-diagonal blocks with the transformations

$$T_{j,\Gamma_{5/6},m_I} = \exp\left(-{\rm i}\phi_{j,\Gamma_{5/6},m_I} \sigma^y_{j,\Gamma_{5/6}}\right) |m_I\rangle \langle m_I|, \text{ with } \tan(2\phi_{j,\Gamma_{5/6},m_I}) = \frac{a^{\perp}_{j,\Gamma_{5/6}} m_I}{\mu_B B g^{\parallel}_{j,\Gamma_{5/6}} + a^{\parallel}_{j,\Gamma_{5/6}} m_I}; \tag{S14}$$

$$\begin{aligned} T_{j,\Gamma_4,m_I} &= \exp\left[-i\phi_{j,\Gamma_4,m_I}(-i |j, \Gamma_4, \uparrow\rangle |m_I\rangle \langle m_I - 1| \langle j, \Gamma_4, \downarrow| + \text{h.c.})\right], \\ \text{with } \tan 2\phi_{j,\Gamma_4,m_I} &= \frac{a^{\perp}_{j,\Gamma_4} \sqrt{I(I+1) - m_I(m_I - 1)}}{\mu_B g^{\parallel}_{j,\Gamma_4} B + a^{\parallel}_{j,\Gamma_4}(m_I - 1/2) + \mu_N g_N B + a^{\rm od}_j 2m_I}; \end{aligned} \tag{S15}$$

TABLE S1. Hyperfine tensors for our model calculated using the fit values of Wolfowicz *et al.* [S2] the defect type assignment in brackets is according to the ab initio results by A. Csóré *et al.*. We omit the errors for the $\Gamma_{5/6}$, because we can directly calculate [see Eq. (S20)] the values from their fit data such that there is no additional error due to fitting.

| Irrep | Crystal | Defect Type | $a^{\perp}_{j,\Gamma_\gamma}/h$ (MHz) | $a^{\parallel}_{j,\Gamma_\gamma}/h$ (MHz) |
|---|---|---|---|---|
| $\Gamma_4$ | 4H-SiC | $\alpha$ (k) | $165.1 \pm 1.7$ | $-232.0 \pm 3.9$ |
| $\Gamma_4$ | 4H-SiC | $\beta$ (h) | $149.5 \pm 4.2$ | $-174.7 \pm 4.3$ |
| $\Gamma_4$ | 6H-SiC | $\alpha$ (k$_2$) | $165.1 \pm 1.6$ | $-232.0 \pm 3.6$ |
| $\Gamma_4$ | 6H-SiC | $\beta$ (k$_1$) | $141.6 \pm 2.4$ | $-171.2 \pm 2.1$ |
| $\Gamma_4$ | 6H-SiC | $\gamma$ (h) | $147.3 \pm 14.5$ | $-175.4 \pm 13.6$ |
| $\Gamma_{5/6}$ | 4H-SiC | $\beta$ (h) | 202.5 | 158.2 |
| $\Gamma_{5/6}$ | 6H-SiC | $\beta$ (k$_1$) | 197.6 | 165.8 |
| $\Gamma_{5/6}$ | 6H-SiC | $\gamma$ (h) | 205.9 | 166.8 |

$$T_{3,\Gamma_4,m_I} = \exp\left[-i\phi_{3,\Gamma_4,m_I}(-i\,|3,\Gamma_4,\uparrow\rangle\,|m_I\rangle\,\langle m_I+1|\,\langle 3,\Gamma_4,\downarrow| + \text{h.c.})\right],$$
$$\text{with}\ \tan 2\phi_{3,\Gamma_4,m_I} = \frac{a^{\perp}_{3,\Gamma_4}\sqrt{I(I+1)-m_I(m_I+1)}}{\mu_B g^{\parallel}_{3,\Gamma_4}B + a^{\parallel}_{3,\Gamma_4}(m_I+1/2) - \mu_N g_N B}. \tag{S16}$$

The corresponding eigenvalues are ($\Gamma_{5/6}$)

$$E_{j,\Gamma_{5/6},\pm,m_I} = E_{j,\Gamma_{5/6}} \pm \frac{\mu_B B g^{\parallel}_{j,\Gamma_{5/6}} + a^{\parallel}_{j,\Gamma_{5/6}} m_I}{2\,|\cos 2\phi_{j,\Gamma_{5/6},m_I}|} + \mu_N g_N m_I B + a^{\text{od}}_j\left[I(I+1) - m_I(m_I+1)\right] \tag{S17}$$

$$E_{j,\Gamma_4,\pm,m_I} = E_{j,\Gamma_4} + \frac{a^{\parallel}_{j,\Gamma_4}}{4} \pm \frac{\mu_N g_N B + a^{\parallel}_{j,\Gamma_4}(m_I - 1/2) + \mu_B g^{\parallel}_{j,\Gamma_4} B}{2\,|\cos 2\phi_{j,\Gamma_4,m_I}|} + \mu_N g_N B(m_I - 1/2) \tag{S18}$$

$$E_{3,\Gamma_4,\pm,m_I} = E_{3,\Gamma_4} - \frac{a^{\parallel}_{3,\Gamma_4}}{4} \pm \frac{\mu_B g^{\parallel}_{3,\Gamma_4} B + a^{\parallel}_{3,\Gamma_4}(m_I + 1/2) - \mu_N g_N B}{2\,|\cos 2\phi_{3,\Gamma_4,m_I}|} + \mu_N g_N B(m_I + 1/2) \tag{S19}$$

## HYPERFINE TENSORS FOR EXPERIMENTAL DATA FROM WOLFOWICZ *ET AL.* [S2]

We compared our model briefly to data by Wolfowicz *et al.* [S2] in the main text; here we provide Table S1 with the least square fits for $\Gamma_4$ defects to translate their model to our model as well as the parameters for $\Gamma_{5/6}$ defects that can be calculated directly using their principal axis tilt $\theta$ and $A_{ZZ}$ ($a^z_{j,\Gamma_{5/6}}$ with $j = 1, 2$ in our notation) value,

$$a^{\perp}_{j,\Gamma_\gamma} = \sin(\theta)A_{ZZ} \qquad\qquad a^{\parallel}_{j,\Gamma_\gamma} = \cos(\theta)A_{ZZ} \tag{S20}$$

. The fit with the worst agreement is for the $\gamma$ site of 6H-SiC, we want to stress that in this case the data provided in the Supplemental Material in [S2] seems to be not described perfectly by their model, too. As this defect configuration also has the smallest $\Delta^{\text{so}}_1$ it would be reasonable to include the second order when fitting to the raw data. The signs in the table carry no physical meaning here, because we did not choose a particular orientation of the $z$-axis, i.e. we do not now the stacking order of the crystal with regard to the direction of the $z$-axis and inverting the magnetic field $B_z \to -B_z$ corresponds to changing the sign of $a^{\parallel}_{j,\Gamma_\gamma}$ in the isolatet KD hyperfine energy lines. The sign of the off-diagonal elements in comparison to the diagonal elements has no effect on the energy levels used in the fit.

---

* benedikt.tissot@uni-konstanz.de
† guido.burkard@uni-konstanz.de
[S1] B. Tissot and G. Burkard, Spin structure and resonant driving of spin-1/2 defects in SiC, Phys. Rev. B **103**, 064106 (2021).
[S2] G. Wolfowicz, C. P. Anderson, B. Diler, O. G. Poluektov, F. J. Heremans, and D. D. Awschalom, Vanadium spin qubits as telecom quantum emitters in silicon carbide, Sci. Adv. **6**, eaaz1192 (2020).
